# Supplementary material for: Covering Tours and Cycle Covers with Turn Costs: Hardness and Approximation
Source: arXiv:1808.04417 source file (2019-04-25)
Supplement: Supplementary file 1 [file 99_appendix.tex]

\section{Details on Integer Programming}
\label{sec:app:ip}
%\todoi{This text is mainly copied and slightly adapted from my thesis}
We provide further details on an integer programming formulation for solving the full coverage tour problem to optimality.
The IP in Eq.~(\ref{eq:obj}) to (\ref{eq:ip:constr2}) described in Sec.~\ref{sec:short_strip_cover} 
already provides a powerful IP formulation for the cycle cover problem.
We experimented with different formulations; this turned out to be the best for most cases and variants. % (but not all).
It is analogous to the cycle cover formulation used by Maurer~\cite{maurer2009diploma}; in order to make it useful
for tours, it only lacks constraints for subtour elimination.
These subtour elimination constraints are more complicated than for the classic TSP, because here 
cycles can intersect without being connected.
% (an implicit connecting would involve additional turns).
We describe two different variants: a simple but insufficient one analogous to the one for TSP, and a more complex one that is sufficient.

\subsection{A Necessary Family of Simple Subtour Separation Constraints}
Let $C$ be a subtour that is not crossed by any other cycle.
It is easy to see that there has to be a variable used that allows to leave the set of pixels $P'=\{p_i\in C\}$ covered by $C$.

\begin{eqnarray}
	\displaystyle \sum\limits_{p_j\in P', i,k\in N(p_j), p_i\not\in P'} x_{ijk}\geq 1  & \forall P'\subsetneq P, P'\not=\emptyset
\end{eqnarray}

This is valid for any real non-empty subset $P'\subsetneq P$ of pixels,
independent of any cycle. Therefore, $C$ may also consist of, e.g., two
intersecting cycles, as long as $C$ does not fully cover all pixel $P$.
This constraint forces cycles to intersect but the turn costs prevent us from assuming that this is sufficient for connecting the cycles.
For example the two cycles in Fig.~\ref{fig:gg:ip:fc:form1:cut2} intersect and hence fulfill aboves constraint but connecting them would cost us two extra turns.
%\todoi{Explain more clearly why this is insufficient.}

\subsection{A Sufficient Family of Advanced Subtour Separation Constraints}
The following separation constraint is valid for all subtours $C$ that have a pixel $p_f$ only covered by $C$ and another pixel $p_{f'}$ not covered by $C$.
For cycle covers that do not already contain a tour, you can argue the existence of such pixels by using the corner pixels which can only be covered by one cycle (as they automatically connect all their cycles).
%Such two pixels do not need to exist for all cycles of a (not necessarily optimal) cycle cover (e.g. if it consists of two tours), 
%\todoi{Why not?}
%but in every cycle cover that does not contain a tour there is at least one such cycle.
The separation constraint enforces that either $p_f$ is passed differently, or there is a turn in a pixel traversed without a turn by $C$, 
or a currently unused variable is used in one of the other pixels of $C$.
Let $F_s$ be the set of pixels different from $p_f$ that are traversed without a turn by $C$. 
Other cycles may also pass pixels in $F_s$, but not by a simple turn as otherwise they would be connected with $C$.
Let $T(p_i)$ be the simple turn variables for the pixel $p_i\in P$ and let $x'$ denote the value of a variable in the current solution.

\begin{equation}
	\sum_{i,j\in N(p_f), x'_{ifj}=0} x_{ifj} + \sum_{t\in T(p_i), p_i\in F_s} t + \sum_{ p_j\in C\setminus (F_s\cup\{p_f\}), i\not=k\in N(p_j), x'_{ijk}=0} x_{ijk} \geq 1
\end{equation}

An example of this separation constraint can be seen in Fig.~\ref{fig:gg:ip:fc:form1:cut2}.
While for the previous separation constraint, we could theoretically use any subset of pixels, this separation constraint needs a preliminary 
solution to be useful for separation.

\begin{figure}
	\centering
	%	\resizebox{0.6\textwidth}{!}{%
	%		\begin{tikzpicture}
	%			\newcommand{\tikzsquare}[3]{ \draw[#3] (#1-0.5,#2-0.5) -- (#1+0.5,#2-0.5) -- (#1+0.5,#2+0.5) -- (#1-0.5, #2+0.5) -- (#1-0.5,#2-0.5); }
	%			\newcommand{\tikzsquares}[5]{ \foreach \a in {#1,...,#3}{ \foreach \b in {#2,...,#4}{ \tikzsquare{\a}{\b}{#5} } } }
	%			\newcommand{\nscut}[2]{ \draw[red] (#1, #2+0.5) -- (#1, #2-0.5); }
	%			\newcommand{\ewcut}[2]{ \draw[red] (#1+0.5, #2-0.05) -- (#1-0.5, #2-0.05); }
	%			\newcommand{\swcut}[2]{ \draw[red] (#1-0.5, #2-0.05) -- (#1-0.05, #2-0.05) -- (#1-0.05, #2-0.5); }
	%			\newcommand{\secut}[2]{ \draw[red] (#1+0.5, #2-0.05) -- (#1+0.05, #2-0.05) -- (#1+0.05, #2-0.5); }
	%			\newcommand{\necut}[2]{ \draw[red] (#1+0.5, #2+0.05) -- (#1+0.05, #2+0.05) -- (#1+0.05, #2+0.5); }
	%			\newcommand{\nwcut}[2]{ \draw[red] (#1-0.5, #2+0.05) -- (#1-0.05, #2+0.05) -- (#1-0.05, #2+0.5); }
	%			\newcommand{\straightcut}[2]{ \nwcut{#1}{#2} \necut{#1}{#2} \secut{#1}{#2} \swcut{#1}{#2}}

	%			\tikzsquares{1}{1}{8}{2}{fill=gray!20}
	%			\tikzsquares{3}{0}{6}{3}{fill=gray!20}
	%			\straightcut{3}{1}
	%			\straightcut{3}{2}
	%			\straightcut{6}{2}
	%			\straightcut{6}{1}
	%			\necut{4}{0} \nwcut{4}{0}
	%			\necut{5}{0} \nwcut{5}{0}
	%			\secut{4}{3} \swcut{4}{3}
	%			\secut{5}{3} \swcut{5}{3}

	%			\draw[fill=black] (3,0) circle (0.1);
	%			\draw[red] (2.95, 0.5) -- (2.95, 0.2) -- (3.05, 0.2) -- (3.05, 0.5);
	%			\draw[red] (3.5, 0.05) -- (3.2, 0.05) -- (3.2, -0.05) -- (3.5, -0.05);

	%			\draw[green, dashed] (1,1) -- (1,2) -- (8,2) -- (8,1) -- cycle;
	%			\draw[blue, dashed] (3,0) -- (3,3) -- (6,3) -- (6,0) -- cycle;

	%		\end{tikzpicture}
	%	}%
		\includegraphics[width=0.4\textwidth]{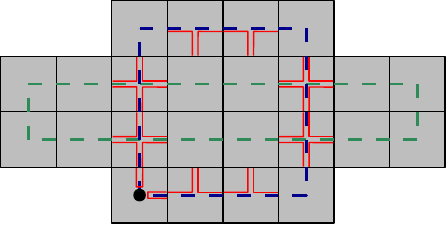}
		\caption[Second subtour separation constraint]{The blue and the green cycle are intersecting and thus the first separation constraint is satisfied even though the two cycles are not connected. We can use the second separation constraint to force the cycles to connect using the black dotted pixel as $p_f$. The constraint forces at least one of the red traversals to be used.}
		\label{fig:gg:ip:fc:form1:cut2}
\end{figure}

\section{Benchmark Examples and Runtime}
\label{sec:app:exp}

\begin{figure}[h]
	\centering
	\includegraphics[width=0.6\textwidth]{./figures/gg_op_n138_s3_scale0_5_7684}
	\caption{An example instance of Type~I with \num{7684} pixels.}
	\label{fig:instanceexample:ortho}
\end{figure}

\begin{figure}
	\centering
	\includegraphics[width=0.9\textwidth]{./figures/gg_rect_n10000_s10052_scale5_10052} 
	\caption{An example instance of Type~IIa with \num{10052} pixels.}
	\label{fig:instanceexample:rect5}
\end{figure}

\begin{figure}
	\centering
	\includegraphics[width=0.9\textwidth]{./figures/gg_rect_n10000_s10004_scale1_10004}
	\caption{An example instance of Type~IIb with \num{10004} pixels.}
	\label{fig:instanceexample:rect1}
\end{figure}

\begin{figure}
        \centering
        \includegraphics[width=0.9\textwidth]{./figures/experiments/scatterplot_cc_apx_runtime.pdf}
        \includegraphics[width=0.9\textwidth]{./figures/experiments/scatterplot_cc_apx_runtime_large.pdf}
        \caption{Runtime of the cycle cover approximation algorithm for Type~I, Type~IIa, Type~IIb and
different turn cost coefficients, indicating the relative cost of a simple turn vs.~a pixel transition.
{\bf (Top)} Instances with up to \num{100000} pixels for all types. 
{\bf (Bottom)} Very large instances with more than \num{300000} pixels for Type~I. 
%Note that the complexity for instances of Type~I is limited such that they only scale in size for large instances while the complexity for instances of Type~II grows with its size. Further, due to the creation process which only takes a boundary complexity and a scale as input, the size distribution of instances of Type~I is not uniform: there are more smaller than larger instances (for Type~II the size distribution is uniform).
}
        \label{plot:runtime}
\end{figure}
